# Supplementary material for: Exact Penalty Method for Variationally Coherent Stochastic Programming Problems
Source: arXiv:2603.25815 source file (2026-06-30)
Supplement: Supplementary file 1 [file appendix.1.kkt.tex]

% We consider the nonlinear programming problem:
% \begin{eqnarray}
% &{\displaystyle \min_{x\in \X} f(x)}       \label{consP1} \\
% &{\displaystyle h_i(x) = 0,\ \ i\in E}     \label{consP21} \\
% &{\displaystyle g_j(x) \leq 0,\ \ j\in I} \label{consP3}
% \end{eqnarray}

% We assume that the set $\X$ is convex and compact, functions $f,\ h_i,\ g_j:\R^n\rightarrow \R$ are continuously differentiable and the sets of indices $E,\ I$ are finite.

In this section, we show proofs of lemmas, propositions and theorems related to constraint qualification conditions.

\subsection{Lemma}

We present the proof of the lemma \ref{l2}.

\begin{lemma}\label{l2}
Assume ${\bf (CQ)}$. For any $\tilde{x}\in\X$, $\varepsilon > 0$,
there exist a neighborhood $\cN(\tilde{x}, \varepsilon)$ of $\tilde{x}$, $K_1, K_2, K_3, K_4, K_5 > 0$, with the following properties: given any 
$x\in \X$ such that $x\in\cN(\tilde{x},\varepsilon)$ there exist $v\in \X$ and $w\in \X$ such that
\begin{align}
\der{h}{x}{v - x} & = -K_1 h(x)/M(x)    \label{CQ1} \\
\der{h}{x}{v - x} & = -K_1 h(x)/M(x)    \label{CQ1} \\
\der{g}{x}{v - x} & = -K_2              \label{CQ2} \\
\mmax{\abs{ h(x) + \der{h}{x}{w - x} }} - \mmax{\abs{h(x)}}
& \leq - K_3 M(x) \label{CQ3} \\
\mmax{\abs{\der{g}{x}{w - x}}} \leq  -K_4 M(x)
\label{CQ4} \\
\norm{ w - x }_{\cL^\infty} \leq \ \ K_5 M(x).
\label{CQ5}
\end{align}
where
\begin{equation}
M(x) = \max \left \{ \mmax{g(x)}, \mmax{\abs{h(x)}} \right \}. \label{CQ6}
\end{equation}
\end{lemma}

\begin{proof} Let $r > 0$ be a number such that
% Take any $x\in \X$.
\begin{equation*}
    M(x) < r
\end{equation*}
for all $x\in \X$. 
\begin{equation*}
\end{equation*}
%	Here,
%	\begin{eqnarray}
%	&{\displaystyle M(x) = \max_{i\in E}|h_i(x)|.}\nonumber
%	\end{eqnarray}
We deduce from ${\bf (CQ)}$ that there is a simplex
in $\cE(x) = \der{h}{x}{\F(x)} \subset
\X^{n_E}$ with vertices $\{e_j\}_{j=0}^{n_E}$ which contains $0$
as an interior point. By definition of $\cE(x)$, there exist
$d_0,\ldots,d_{n_E}\in \D$ and $\delta > 0$ such that for $j=0,\ldots,n_E$
% \begin{equation*}
% \left \{ \left \langle \nabla h_i(x),
% d_j\right \rangle\right \}_{i\in E} =  e_j,\ \ 
% \max_{i\in I} \left \langle \nabla h^2_i(x),
% d_j \right \rangle  \leq  - \delta.
% \end{equation*} 
\begin{equation*}
\der{h}{x}{d_j} =  e_j,\ \ 
\der{h}{x}{d_j} \leq  - \delta.
\end{equation*}
Let $(\lambda_0,\lambda_1,\ldots,\lambda_{n_E})$ be the barycentric coordinates of $0$
w.r.t. the vertices $e_j$ of the simplex, i.e.
\begin{equation*}
0 = \sum_{j=0}^{n_E} \lambda_j e_j = \der{h}{x}{\sum_{j=0}^{n_E} \lambda_j d_j}.
\end{equation*}
Since the vertices are in general position and $0$ is an interior point, the $\lambda_i$'s are all positive and we may find $\delta_1 > 0$ such that for all $\alpha\in \B(0,\delta_1)\subset \X^{n_E}$:
\begin{equation}
\begin{split}
    \left(
        \lambda_0 - \sum_{j=1}^{n_E} \alpha_j,
        \lambda_1 + \alpha_1,
        \ldots, \lambda_{n_E} + \alpha_{n_E}
    \right) \nonumber \\
\in \left \{ \gamma\in \X^{n_E+1}:\ \gamma_j \geq 0\ \forall
j,\ \sum_{j=0}^{n_E}\gamma_j =1 \right \}
\nonumber
\end{split}
\end{equation}
($\B(0,\delta_1)$ is a ball with radius $\delta_1$.)
Furthermore, the $n_E\times n_E$ matrix $P(x)$
defined by
\begin{equation}
P(x)\alpha := \sum_{j=1}^{n_E} \nabla h(x)\circ \alpha_j (d_j-d_0)
\label{b1}
\end{equation}
\begin{equation}
P(x)\alpha :=\der{h}{x}{\sum_{j=1}^{n_E} \alpha_j (d_j-d_0)}
\label{b1}
\end{equation}
\begin{equation}
P(x)\alpha :=\der{h}{x}{\sum_{j=1}^{n_E} \alpha_j d_j - \sum_{j=1}^{n_E} \alpha_j d_0}
\label{b1}
\end{equation}
\begin{equation}
P(x)\alpha :=\der{h}{x}{d \alpha - \left(
    \sum_{j=1}^{n_E} \alpha_j 
\right) d_0}
\label{b1}
\end{equation}
\begin{equation}
P(x)\alpha :=\der{h}{x}{d \alpha - (1^T \alpha ) d_0}
\label{b1}
\end{equation}
\begin{equation}
P(x)\alpha :=\der{h}{x}{d \alpha - (d_0 1^T) \alpha }
\label{b1}
\end{equation}
\begin{equation}
P(x)\alpha :=\der{h}{x}{(d  - (d_0 1^T)) \alpha }
\label{b1}
\end{equation}
\begin{equation}
P(x) :=\der{h}{x}{} \circ (d  - (d_0 1^T)) = \der{h}{x}{d  - (d_0 1^T)}
\label{b1}
\end{equation}
is invertible for $x=\tilde{x}$, from the definition of $d_j,\ j= 1,\ldots,n_E$.

In consequence of hypothesis ${\bf (CQ)}$ we may choose a neighborhood $\cN(\tilde{x},\varepsilon)$ ($\varepsilon > 0$) of $\tilde{x}$ in $\X$ and
numbers 	$\hat{r}\geq r$ and $\delta_2\in (0,\hat{r}^{-1}]$ such that for any
$x\in \X$ satisfying $x\in \cN(\tilde{x},\varepsilon)$
\begin{align}
&
(i) \max_{i\in I} \der{g_i}{x}{v_j - x} \leq
- \delta/2\ \ \forall j   \nonumber
\\ &
(i) \max_{i\in I} \der{g_i}{x}{v_j - x} \leq
- \delta/2\ \ \forall j \nonumber
\\ & 
(ii) P(x)\ \ {\rm is\ invertible} \nonumber
\\ &
(iii) \left \| P(x)^{-1} \nabla c(x)\circ
\left (\left (\sum_{j=0}^{n_E} \lambda_j v_j\right )-x\right )
\right \| \leq \delta_1/2\nonumber
\\ &
(iv) \delta_2 \left \| P(x)^{-1} 
\right \| n_E^{1/2} \leq \delta_1/2 .\nonumber
\end{align}
(In {\it (iv)} the norm is the Frobenius norm.
Here the controls $v_j\in \X$, $j=0,\ldots,n_E$ are defined to be
\begin{eqnarray}
&{\displaystyle
	v_j:= x + d_j(x).}\nonumber
\end{eqnarray}

Now suppose that the control $x$ is not feasible.
Set
\begin{eqnarray}
&{\displaystyle
	\alpha = P(x)^{-1} \left [ - \nabla c(x)\circ
	\left (\left (\sum_{j=0}^{n_E}\lambda_j v_j\right ) -x\right )
	- \delta_2 M(x)^{-1}
	c(x) \right ]. }
\nonumber \\
\label{b2}
\end{eqnarray}
%in which $\| h_i(x)\|_{\infty} := \max_{i\in E}
%|h_i(x)|$. 
Notice that, by properties {\it (iii)} and {\it (iv)},
$\| \alpha \| \leq \delta_1$. Also set
\begin{eqnarray}
&{\displaystyle
	\hat{v} = v_0 + \sum_{j=1}^{n_E} (\lambda_j + \alpha_j)(v_j-v_0).}\nonumber
\end{eqnarray}
Because $\| \alpha \| \leq \delta_1$ we have that $\hat{v}\in \X$.
Finally we define $v$ to be
\begin{eqnarray}
&{\displaystyle
	v = x + \left (M(x)/\hat{r}\right )(\hat{v}-x).}\nonumber
\end{eqnarray}
Since $M(x)/\hat{r} \leq 1$, it follows that
$v\in \X$.

\medskip

We now verify that this control function has the required
properties.                     

\begin{itemize}
\item[5.]
Notice first that
\begin{equation}
\left \| v - x \right \|_{{\mathcal L}^\infty} \leq (2d/\hat{r})M(x), \label{b3}
\end{equation}
where $d$ is a bound on the norms of elements in $\X$.

\item[3.]
We have from (\ref{b1}) and (\ref{b2}) that
\begin{equation}
\begin{split}
    P(x)\alpha = \nabla h(x)\circ \sum_{j=1}^{n_E}  \alpha_j(v_j- v_0) 
\\
    = - \nabla h(x)\circ \left( \sum_{j=1}^{n_E} \lambda_j \left( v_j - v_0 \right) 
    + v_0 - x \right) - \delta_2 M(x)^{-1} h(x).
\end{split} \nonumber
\end{equation}
By definition of $\hat{v}$,
\begin{equation*}
    \nabla h(x)\circ (\hat{v}-x) = -\delta_2 M(x)^{-1}h(x).
\end{equation*}
But then
\begin{equation*}
    \nabla h(x)\circ (v - x) = -(\delta_2/
    \hat{r})h(x).
\end{equation*}
Since $\delta_2/\hat{r}\leq 1$, it follows that
	\begin{eqnarray}
	&{\displaystyle
		\max_{i\in E} \left | \bar{g}^1_i(u) + \left \langle \nabla \bar{g}^1_i(u),
		v-u\right \rangle \right |
		- \max_{i\in E} \left | \bar{g}^1_i(u)\right |
		\leq - (\delta_2/\hat{r})M(u).}\label{b4}
	\end{eqnarray}

\item[2.]
We deduce from property {\it (i)} that
\begin{equation}
	\left \langle \nabla g_j(x),v_0 + \sum_{i=1}^{n_E}\left (\lambda_i +
	\alpha_i\right )\left (v_i-v_0\right )-x\right \rangle 
	\leq - \delta/2,\ \forall j\in I.
    \nonumber
\end{equation}
It follows that
\begin{eqnarray}
    \left \langle \nabla g_j(x),v-x\right \rangle \leq \left (M(x)\right )\left ( -
	\delta/2\right )\ \forall j\in I.
    \nonumber
\end{eqnarray}

\item[4.]
Since $M(x)/\hat{r}\leq 1$ 
we deduce that
\begin{equation*}
	\min\left [0,g_j(x)\right ]+
	\left \langle \nabla g_j(x), v-x\right \rangle \leq 
	-\left (\delta/\left (2\hat{r}\right )\right )M(x)\ \forall j\in I.
\label{b5}
\end{equation*}
\end{itemize}

Surveying inequalities (\ref{b3})--(\ref{b5}),
we see that $v$ satisfies all relevant
conditions for completion of the proof, 
when we set $K_1 = \min \{\delta_2,\delta/(2\hat{r})\}$
and $K_2 = 2d/\hat{r}$,
numbers whose magnitudes do not depend on our choice of $u$.

\end{proof}

% \newpage
% \subsection{Pietrzykowski's lemma}
% \input{appendix.pietrzykowski_proof}

\newpage
\subsection{Main Theorem}

Using {\it Lemma \ref{l2}} and {\it Lemma \ref{pl}} we can prove the theorem \ref{t1p}.

\begin{theorem}\label{t1p}
Suppose that functions $f$, $h_i$, $i\in E$, $g_j$, $j\in I$ are continuously differentiable on the neighborhood of the point $\bar{x}$ on which the point is the strict local minimum of the problem ${\bf (C)}$ (which means that $\bar{x}$ is feasible with respect to all constraints, in particular $\bar{x}\in \X$) and that at the point $\bar{x}$ constraint qualification ${\bf (CQ)}$ holds. Then for each norm $\|\cdot\|$ in $\X^n$ there exists an $\bar{p} > 0$ such that for all $p\geq \bar{p}$ a local minimum $\bar{x}$ is a local minimum of $P(x,p)$ on the set $\X$. 
\end{theorem}

\begin{proof}
For the simplicity of presentation we assume that $I = \emptyset$ and that the norm in $P$ is $l_1$ norm. One can refer to \cite{Han} (Theorem 4.2 (Equality of local solutions of exact penalty functions)) in order to verify the claim that the norm choice is not important from the theorem thesis perspective. The proof goes along the lines of the proof of Theorem 4.4 in \cite{Han}.

Suppose that $\bar{x}$ is the strict local minimum of the problem ${\bf (C)}$ in the set $\cN(\bar{x},\bar{\varepsilon})\cap$  $\X$, $\bar{\varepsilon} > 0$. According to {\it Lemma \ref{pl}} for sufficiently large values of $p$ there exist $\varepsilon (p) > 0$ and $x(p)$ such that $x(p)$ is a local minimum of the problem ${\bf (U)}$ in the set $\cN(\bar{x},\varepsilon (p))\cap \X$. Since $\varepsilon (p) \rightarrow_{p\rightarrow \infty}  0$ we can choose $p$ sufficiently large so that we will have $\varepsilon (p) \leq \bar{\varepsilon}$. Suppose that $x(p)$ is feasible with respect to the constraints $c(x) = 0$. The we will have
\begin{eqnarray}
&{\displaystyle P(x(p),p) = f(x(p)) \leq P(\bar{x},p) = f(\bar{x}),} \nonumber
\end{eqnarray}
which means that we must have $x(p) = \bar{x}$ since $\bar{x}$ is a strict local minimizer in the set $\cN(\bar{x},\varepsilon (p))\cap \X$ so it is the only minimizer in the set. This means $\bar{x}$ is the local minimizer for the problem ${\bf (U)}$ in the set $\cN(\bar{x},\varepsilon (p))\cap \X$.

Therefore, we have to show that for sufficiently large values of $p$ vectors $x(p)$ will be feasible with respect to constraints $c(x) = 0$. Suppose that it is not true, thus for any $p\rightarrow \infty$ there exists an index $i_p\in E$ such that $h_{i_p}(x(p)) \neq 0$.  Since at $\bar{x}$ ${\bf (CQ)}$ holds there exists a neighborhood $\cN(\bar{x},\varepsilon_1)$, $\varepsilon_1 > 0$ such that for any $x\in \cN(\bar{x},\varepsilon_1)$ there exists $v\in \X$ and $K_1 > 0$ with the property
\begin{eqnarray}
&{\displaystyle \left \langle \nabla h_i(x),v- x\right \rangle   =  -K_1 h_i(x)/M(x),\ i\in E.      }\nonumber 
\end{eqnarray}

Suppose that $\bar{i}_p(x) \in E$ is such that $\left |h_{\bar{i}_p(x)} (x) \right | = M(x)$ (notice that we have assumed that $I = \emptyset$). Then we have
\begin{eqnarray}
&{\displaystyle  \left \langle \nabla h_i(x),v- x\right \rangle = \left \{ 
	\begin{array}{ll}
	-K_1 & {\rm if}\ i=\bar{i}_p(x)\ \ {\rm and}\ h_{\bar{i}_p}(x) = M(x) \nonumber \\
   K_1   & {\rm if}\ i=\bar{i}_p(x)\ \ {\rm and}\ h_{\bar{i}_p}(x) = - M(x) \nonumber \\                   
   -K_1 |h_i(x)|/M(x) & {\rm if}\ h_i(x) \geq 0 \nonumber \\
   K_1 h_i(x)/M(x) & {\rm if}\ h_i(x) < \leq 0 \nonumber
   \end{array} 
   \right. .} \label{ep1}                
 \end{eqnarray}
 
For sufficiently large $p$ $x(p)\in \cN(\bar{x},\varepsilon_1)$ and $x(p)$ is not feasible with respect to constraints $c(x) = 0$. From {\it Lemma \ref{l2}} for any $p$ there exists $v \in \X$ such that the directional derivative of $P(x,p)$ in the direction $v-x$ can be evaluated according to the formula (notice that we consider $l_1$ norm in the definition of $P$):
\begin{eqnarray}
&{\displaystyle 
DP(x,p;v-x) = \left \langle \nabla f(x),v-x \right \rangle + p \sum_{h_i(x) > 0,i\neq \bar{i}_p(x)} \left \langle \nabla h_i(x),v-x \right \rangle }\nonumber \\
&{\displaystyle -p \sum_{h_i(x) < 0,i\neq \bar{i}_p(x)} \left \langle \nabla h_i(x),v-x \right \rangle  + p \sum_{h_i(x) =0} \left |\left \langle \nabla h_i(x),v-x \right \rangle \right |  }\nonumber \\
&{\displaystyle + p \sum_{i = \bar{i}_p(x), h_i(x) >0} \left \langle \nabla h_i(x),v-x \right \rangle -
p \sum_{i = \bar{i}_p(x), h_i(x) <0} \left \langle \nabla h_i(x),v-x \right \rangle
.} \nonumber
\end{eqnarray}

From (\ref{ep1}) it follows that
\begin{eqnarray}
&{\displaystyle DP(x,p;v-x) = \left \langle \nabla f(x),v-x \right \rangle - K_1 p \leq  \|\nabla f(x) \| \|v-x \| - K_1p. }\label{ep2}
\end{eqnarray}
Furthermore, for sufficiently large values of $p$ we have that $x(p)\in \cN(\bar{x},\varepsilon_1)$ and at the same time, from (\ref{ep2}),
\begin{eqnarray}
&{\displaystyle DP(x(p),p;v-x(p)) < 0} \label{ep3}
\end{eqnarray}
and, since $v\in \X$, (\ref{ep3}) contradicts the assumption that $x(p)$ is a local minimizer of the problem ${\bf (U)}$. It means that for sufficiently large values of $p$ $x(p)$ is feasible with respect to the constraints $c(x) = 0$.

\end{proof}

Using parts of the proof of {\it Theorem \ref{t1p}} we are able to prove the following theorem.
\begin{theorem}[Strict Local Minimizer]\label{t2p}
Suppose that functions $f$, $h_i$, $i\in E$, $g_j$, $j\in I$ are continuously differentiable on the neighborhood of the point $\bar{x}$ and that constraint qualification holds at any $x\in \X$. Then there exists an $\bar{p} > 0$ such that for all $p\geq \bar{p}$, if $\bar{x}$ is a strict local minimum point of the problem ${\bf (U)}$ then $\bar{x}$ is also a strict local minimum point of the problem ${\bf (C)}$.  
\end{theorem}

\begin{proof}
In the proof of {\it Theorem \ref{t1p}} we showed that under constraint qualification, if $\bar{x}$ is a strict local minimum point of the problem $\bf{(U)}$ it is also a feasible point as far as constraints of the problem $\bf{(C)}$ are concerned. It means that for all $x\in \cN(\bar{x},\varepsilon(p))\cap \X$, $x\neq \bar{x}$ and $p\geq \bar{p}$
\begin{equation}
f(\bar{x}) = P(\bar{x},p) < P(x,p)
\end{equation}
which implies that
\begin{equation}
%\forall x \in \cN(\bar{x},\varepsilon(p))\cap \X\cap \cG,\ x\neq \bar{x},\ p\geq \bar{p}, \label{ep4}
h(x) = 0, \ g(x)\leq 0 \implies f(\bar{x}) = P(\bar{x},p) <  P(x,p) = f(x)
\end{equation}
But (\ref{ep4}) states that $\bar{x}$ is a strict local minimum for the problem ${\bf (C)}$.
\end{proof} 

\newpage
\section{KKT conditions for problems (C) and (U)}

In order to derive necessary optimality conditions for the problem ${\bf (C)}$ we have to introduce the definition of the tangent cone to the set $\cY$.
\newtheorem{d1}{Definition}%[section]
\begin{d1}
\label{d1}
Suppose that $\cY\subset \X^n$ is nonempty. We say that a direction $d\in \X^n$ is tangent to $\cY$ at $x\in \cY$ if there exist sequences $\{x_k\}$ and $\{t_k\}$ such that
\begin{eqnarray}
    &{\displaystyle x_k\rightarrow x,\ \ t_k \downarrow 0,\ \ \frac{x_k -x}{t_k} \rightarrow d.} \label{ld1}
\end{eqnarray}

The set of all tangent directions to $\cY$ at $x$ is called the tangent cone and is denoted by $T_\cY(x)$.
\end{d1}

If $\cY$ is a convex set one can provide the following characterization of $T_\cY(x)$.
\newtheorem{ptc1}{Proposition}%[section]
\begin{ptc1}
\label{ptc1}
Suppose that $\cY$ is a compact convex set and $x\in \cY$. Then $T_\cY(x)$ is the closure of the cone generated by $\cY - \{x\}$:
\begin{eqnarray}
    &{\displaystyle T_\cY(x) = {\rm cl}\left \{d\in \X^n:\ \ d=\alpha (y-x),\ y\in \cY,\ \alpha \geq 0\right \}} \label{tc1}
\end{eqnarray}

\end{ptc1}

\newtheorem{d2}[d1]{Definition} % [section]
\begin{d2}
\label{d2}
The direction $s$ is said to be normal to $\cY$ at $x$ if the following holds
\begin{eqnarray}
    &{\displaystyle \left \langle s,y -x\right \rangle \leq 0,\ \ \forall y\in \cY.} \label{ld2}
\end{eqnarray}

The set of all normal directions to $\cY$ at $x$ is called the normal cone and is denoted by $N_\cY(x)$.
\end{d2}

One can prove (see \cite{hl96}).
\newtheorem{ptc2}[ptc1]{Proposition}
\begin{ptc2}
\label{ptc2} The tangent and polar cones share the following properties
\begin{enumerate}
    \item[i)] The tangent cone is the polar of the normal cone: 
    \begin{eqnarray}
        &{\displaystyle T_\cY(x) = \left \{ d\in \X^n:\ \left \langle s,d\right \rangle\leq 0 \ \forall s\in N_\cY(x)\right \}. }\nonumber
    \end{eqnarray}
    \item [ii)] If $\cY_1$, $\cY_2$ are nonempty closed convex sets and $x\in \cY_1\cap \cY_2$, then
    \begin{eqnarray}
        &{\displaystyle T_{\cY_1\cap \cY_2} (x)  \subset T_{\cY_1}(x) \cap T_{\cY_2}(x),\ \ N_{\cY_1\cap \cY_2} \subset N_{\cY_1}(x) + N_{\cY_2}(x)} \nonumber
    \end{eqnarray}
    and the equality holds if 
    \begin{eqnarray}
        &{\displaystyle 0\in {\rm ri} \left ( \cY_1 - \cY_2\right ),\ or,\ \left ({\rm ri}\cY_1\right ) \cap \left ({\rm ri}\cY_2\right )\neq \emptyset } \nonumber
    \end{eqnarray}
    where ${\rm ri} \cC$ is the relative interior of $\cC$.
    \item[iii)] Suppose that $\cC = \{x\in \X^n:\ h_i(x) =0,\ i=1,\ldots,m\}$, where functions $h_i$ are continuously differentiable. If $x\in \cC$ and $\nabla h_i(x)$, $i=1,\ldots,m$ are linearly independent, then
    \begin{eqnarray}
        &{\displaystyle T_\cC(x) = \left \{ d\in \X^n:\ \left \langle \nabla h_i(x),d\right \rangle = 0\right \}.}\nonumber 
    \end{eqnarray}
\end{enumerate}

\end{ptc2}

In order to derive necessary optimality conditions for the problem ${\bf (C)}$ consider the problem
\begin{eqnarray}
    &{\displaystyle \min_{x\in \cY} f(x),}\label{con1}
\end{eqnarray}
where $\cY = \cC\cap \X$, $\cC = \{x\in \X^n:\ h_i(x) = 0,\ i=1,\ldots,m\}$.

One can prove the following results (\cite{hl96}).
\newtheorem{ptc3}[ptc1]{Proposition}
\begin{ptc3}
\label{ptc3}
Suppose that the set $\cY$ is convex and compact, for any $x\in \cY$ there exists subdifferential $\partial f(x)$ and that $\bar{x}$ is a local solution of the problem (\ref{con1}), then the followinh hold
\begin{enumerate}
    \item [i)] $Df(\bar{x};y-\bar{x}) \geq 0$ for all $y\in \cY$;
    \item [ii)] $Df(\bar{x};d) \geq 0$ for all $d\in T_\cY(\bar{x})$;
    \item [iii)] $0\in \partial f(\bar{x}) + N_\cY(\bar{x})$.
\end{enumerate}

\end{ptc3}

Suppose now that the following hold
\begin{align}
    &
    N_\cC(x) = \left \{d\in \X^n:\ d = \sum_{i=1}^m \alpha_i \nabla h_i(x),\ \alpha_i\in \X\right \} 
    \label{con2}
    \\ &
    N_\cY(x) = N_\cC(x) + N_\X(x).
    \label{con3}
\end{align}

If $\bar{x}$ is a local solution to the problem (\ref{con1}) then according to {\it Proposition \ref{ptc3}}, part {\it iii)}, (\ref{con2})--(\ref{con3}) one can write
\begin{eqnarray}
    &{\displaystyle 0\in \partial f(\bar{x}) + \sum_{i=1}^m \bar{\alpha}_i \nabla h_i (\bar{x}) + N_\X(\bar{x}),}\label{con4}
\end{eqnarray}
for some $\bar{\alpha}_i\in \X$, $i=1,\ldots,m$.

Suppose now that $\bar{x}$ is a local solution to the problem ${\bf (U)}$. Then, we have
\begin{eqnarray}
    &{\displaystyle 0\in \partial P(\bar{x},p) + N_\X (\bar{x}).}\label{con5}
\end{eqnarray}

If we denote by $\bar{g} =\left [\bar{g}_1,\bar{g}_2,\ldots,\bar{g}_m\right ]^T$ the subgradient of the norm $\|\cdot\|:\X^m\rightarrow \X$ evaluated at the point $c(\bar{x})$ then we can express (\ref{con5}) by
\begin{eqnarray}
    &{\displaystyle 0\in \partial f(\bar{x}) + \sum_{i=1}^m (p\bar{g}_i) \nabla h_i(\bar{x}) + N_\X(\bar{x}),}\label{con6}
\end{eqnarray}
which is (\ref{con4}) if we substitute $p\bar{g}_i$ for $\bar{\alpha}_i$.

\newpage
