# Supplementary material for: Exact Penalty Method for Variationally Coherent Stochastic Programming Problems
Source: arXiv:2603.25815 source file (2026-06-30)
Supplement: Supplementary file 2 [file appendix.pietrzykowski_proof.tex]

The following results depend on the lemma proved in \cite{Piet}.

\begin{lemma} \label{pl}
Suppose that functions $f$, $h_i$, $i\in E$ and $g_j$, $j\in I$ are continuous on a neighborhood of $\bar{x}$ which is a strict local minimum point of the problem ${\bf (C)}$.
Then there exists $\bar{p} > 0$ such that for any $p\geq \bar{p}$ there exists $\varepsilon (p)$ and a vector $x(p)\in \X^n$ such that 
\begin{enumerate}
	\item [i)] $x(p) \in \cN(\bar{x},\varepsilon (p))\cap \X$
	\item [ii)] $\lim_{p\rightarrow \infty} \varepsilon (p) = 0$
	\item [iii)] $P(x(p),p) \leq P(x,p)$ for all $x\in \cN(\bar{x},\varepsilon(p))\cap \X$.
\end{enumerate}
\end{lemma}
\begin{proof}

Recall the definition of $P(x,p) := f(x) + p\|g(x)_+, c(x)\|$, where $\|\cdot\|$ is any norm. We aim to show, that there exists $\bar{p} > 0$ such that for any $p\geq \bar{p}$ there exists $\varepsilon (p)$ and a vector $x(p)\in \X^n$ such that the above conditions hold true.
% \begin{enumerate}
% 	\item [i)] $x(p) \in \cN(\bar{x},\varepsilon (p))\cap \X$
% 	\item [ii)] $\lim_{p\rightarrow \infty} \varepsilon (p) = 0$
% 	\item [iii)] $P(x(p),p) \leq P(x,p)$ for all $x\in \cN(\bar{x},\varepsilon(p))\cap \X$.
% \end{enumerate} 

\medskip

Let $g(x) := \| g(x)_+, c(x)\|$ and $\F := \{ x \in \mathcal{X} \;|\; g(x) = 0 \}$ denote the feasible set. We will firstly show that $\F$ is closed.
From definition of $g$ it is non-negative, and from continuity of $g$ and $c$ it is also continuous. Therefore, $g^{-1}((0, \infty))$ is open as $(0, \infty)$ is open. Recall that $\mathcal{X}$ is a compact and Hausdorf, hence it is closed and finally $F = \mathcal{X} \setminus g^{-1}((0, \infty))$ is closed as well.

The outline of the proof is as follows:
\begin{enumerate}
    \item Firstly, we prove that:
    \begin{equation}
        \exists_{\delta, p :\; \mathbb{R}_+ \to \mathbb{R}_+}\forall_{\varepsilon \in \mathbb{R}_+} \delta(\varepsilon) < \varepsilon \wedge \left[ \forall_{p \geq p(\varepsilon)} \forall_{x \in S(\bar{x}, \delta(\varepsilon))}P(x, p) > P(\bar{x}, p) \right] \tag{L1}
    \end{equation}
    \begin{enumerate}
        \item $\exists_{\delta: \mathbb{R}_+ \to \mathbb{R}_+}\forall_{\varepsilon \in \mathbb{R}_+} \delta(\varepsilon) < \varepsilon \wedge \inf\{f(x) - f(\bar{x}) \;|\; x \in S(\bar{x}, \delta(\varepsilon)) \cap \mathcal{F}\} > 0$
        \item $\exists_{v : \mathbb{R}_+ \to \mathbb{R}_+} \forall_{\varepsilon \in \mathbb{R}_+}\forall_{v \geq v(\varepsilon)} \forall_{x \in S(\bar{x}, \delta(\varepsilon))}\; [g(x) \geq v \vee f(x) - f(\bar{x}) \geq v]$
        % \\ where $S(\varepsilon) := S(\bar{x}, \delta(\varepsilon))$.
        %P(v, \varepsilon) \cup T(v, \varepsilon)$ 
        %\begin{itemize}
            %\item $S(\varepsilon) := S(\bar{x}, \delta(\varepsilon))$,
            %\item $P(v, \varepsilon) := \{x \in S(\varepsilon) \;|\; g(x) \geq v\}$,
            %\item $T(v, \varepsilon) := \{x \in S(\varepsilon) \;|\; f(x) - f(\bar{x}) \geq v\}$.
        %\end{itemize}
        \item we define $p(\varepsilon) := 2\sup_{x \in S(\bar{x}, \delta(\varepsilon))} |f(x) - f(\bar{x})|  / v(\varepsilon)$, and show that:
        \begin{equation*}
            \forall_{\varepsilon \in \mathbb{R}_+}\forall_{p \geq p(\varepsilon)}\forall_{x \in S(\bar{x}, \delta(\varepsilon))} P(x, p) > P(\bar{x}, p)
        \end{equation*}
    \end{enumerate}
    \item Secondly, we phrase the result in therms of the penalty parameter $p$:
    \begin{equation}\tag{L2}
        \exists_{\varepsilon:\;\mathbb{R}_+ \to \mathbb{R}_+} \lim_{p\to\infty} \varepsilon(p) = 0 \wedge \forall_{p \in \mathbb{R}_+}\forall_{x \in S(\bar{x}, \delta(\varepsilon(p)))} P(x, p) > P(\bar{x}, p) 
    \end{equation}
    \item Finally, we show that:
    \begin{equation}\tag{L3}
        \exists_{x: \mathbb{R}_+ \to \mathcal{X}} \forall_{p \in \mathbb{R}_+} {x(p) \in B(\bar{x}, \delta(\varepsilon(p)))} \wedge \forall_{x \in B(\bar{x}, \delta(\varepsilon(p)))} P(x(p), p) \leq P(x, p)
    \end{equation}
\end{enumerate}

\noindent 1.
We will firstly prove, that for each $\varepsilon > 0$ there exists $p(\varepsilon) > 0$ and $\delta(\varepsilon) > 0$ such that for all $p \geq \bar{p}$ and $x \in S(\bar{x}, \delta (\varepsilon)) \cap \mathcal{X}$:
\begin{eqnarray}
    \delta(\varepsilon) < \varepsilon \quad\text{and}\quad P(x, p) > P(\bar{x}, p).
\end{eqnarray}
\noindent (a)
Let $\F$ denote the feasible set.
The $\bar{x}$ is a strong minimum of $f$ on $\F$, hence there exists $\delta(\varepsilon)$ such that:
\begin{eqnarray}
    \delta(\varepsilon) < \varepsilon \quad\text{and}\quad \inf_{x \in S(\varepsilon) \cap \F} \{f(x)\} > f(\bar{x})
\end{eqnarray}
where $S(\varepsilon) := S(\bar{x}, \delta(\varepsilon)) \cap \mathcal{X}$. 

\medskip

\noindent (b) Now we will prove that there exists $v(\varepsilon) > 0$ such that for all $v \in (0, v(\varepsilon)]$ and $x \in S(\varepsilon)$:
\begin{equation}
    g(x) \geq v
    \quad\text{or}\quad
    f(x) - f(\bar{x}) \geq v
\end{equation}

%\begin{equation}
%    P(v, \varepsilon) \cup T(v, \varepsilon) = S(\varepsilon)
%\end{equation}

%Let us define:
%\begin{eqnarray}
%    P(v, \varepsilon) = \{x \in S(\varepsilon) \;|\; \|g(x)_+, c(x)\| \geq v \} \\ 
%    T(v, \varepsilon) = \{x \in S(\varepsilon) \;|\; f(x) - f(\bar{x}) \geq v \}
%\end{eqnarray}
% \begin{equation} 
%z(u, \varepsilon) \notin P(v(u, \varepsilon), \varepsilon) \cup T(v(u, \varepsilon), \varepsilon)
%\end{equation}
%or equivalently:

\noindent(by contradiction) Suppose it is not true, then for all $u > 0$ there exists $v(u, \varepsilon) \in (0, u]$ and $x(u, \varepsilon) \in S(\varepsilon)$ such that:
\begin{equation}
f(x(u, \varepsilon)) - f(\bar{x}) < v(u, \varepsilon)
\quad\text{and}\quad
g(x(u, \varepsilon)) < v(u, \varepsilon)
\end{equation}
As $v(u, \epsilon) \leq u$ and $g$ is bounded from below by $0$:
\begin{equation}
0 \leq g(x(u, \varepsilon)) < u \quad\text{and}\quad f(x(u, \varepsilon)) - f(\bar{x}) < u
\end{equation}
Since the sphere $S(\bar{x}, \delta(\varepsilon))$ and $\X$ are compact, $S(\varepsilon) = S(\bar{x}, \delta(\varepsilon)) \cap \X$ is also compact. Let $\{u_k\}_{k=0}^\infty$ be a sequence with $u_k > 0$ for all $k$, and $\lim_{k \rightarrow \infty} u_k = 0$. From compactness of $S(\varepsilon)$ there exists subsequence $\{x(u_{k_j}, \varepsilon)\}_{j=0}^\infty$ convergent to a limit point $\tilde{x}$. Because of the continuity of $g$ and $f$, the following limits exist:
\begin{equation}
\lim_{j \rightarrow \infty} g(z(u_{k_j}, \varepsilon)) = g(\bar{z}) \quad\text{and}\quad \lim_{j \rightarrow \infty} f(z(u_{k_j}, \varepsilon)) - f(\bar{x}) = f(\bar{z}) - f(\bar{x})
\end{equation}
we also necessarily have that:
\begin{equation}
g(\bar{z}) = 0 \quad\text{and}\quad f(\bar{z}) - f(\bar{x}) \leq 0
\end{equation}
From $g(\bar{z}) = 0$ the $\bar{z}$ belongs to the feasible set. Since for all $u$ we have $z(u, \varepsilon) \in S(\varepsilon)$, which is closed, $\bar{z} \in S(\varepsilon)$, hence $f(\bar{z}) > f(\bar{x})$ which contradicts $f(\bar{z}) - f(\bar{x}) \leq 0$.

Remark: It would be convenient to define $\lim_{u \downarrow 0} f(u)$ as a set of limit points, i.e., set of limit points of all convergent subsequences. Then we could write without selecting a particular sequence: 
\begin{equation}
\lim_{u \downarrow 0} g(z(u, \varepsilon)) = 0 \quad\text{(meaning forall... = 0) and}\quad \lim_{u \downarrow 0} f(z(u, \varepsilon)) - f(\bar{x}) \leq 0 
\end{equation}
From first we have that $\lim_{u \downarrow 0} z(u, \varepsilon) \subseteq \F$. For all $u$ we have that $z(u, \varepsilon) \in S(\varepsilon)$ which is closed, hence $\lim_{u\downarrow 0} z(u, \varepsilon) \subseteq S(\varepsilon)$
hence $\lim_{u \downarrow 0} f(z(u, \varepsilon)) - f(\bar{x}) > 0$ which contradicts $\lim_{u \downarrow 0} f(z(u, \varepsilon)) - f(\bar{x}) \leq 0$.

\medskip
\noindent \textbf{(c)} Now let:
\begin{equation}
    p(\varepsilon) = \frac{2\sup_{x \in S(\varepsilon)}\{|f(x) - f(\bar{x})|\} + c}{v(\varepsilon)}
\end{equation}
where $c > 0$.
Recall that $v(\varepsilon)$ is positive for each $\varepsilon > 0$. From (a) we know that $f(x) > f(\bar{x})$ for all $x \in S(\varepsilon) \cap \mathcal{F}$, .

Let $p \geq p(\varepsilon)$ and $x$ a point in $S(\varepsilon)$.
%= P(v(\varepsilon), \varepsilon) \cup T(v(\varepsilon), \varepsilon)$.
We showed that either $f(x) - f(\bar{x}) \geq v$ or $g(x) \geq v$, for all $v \in (0, v(\varepsilon)]$. If $g(x) \geq v$ is true, then
\begin{equation}
\begin{split}
    P(x, p) - P(\bar{x}, p) & = f(x) + p g(x) - f(\bar{x}) - p g(\bar{x}) \\
    & = f(x) - f(\bar{x}) + p g(x) \\
    %& \geq f(x) - f(\bar{x}) + pj v(\varepsilon) \\ 
    %& \geq f(x) - f(\bar{x}) + p(\varepsilon) v(\varepsilon) \\ 
    & \geq -|f(x) - f(\bar{x})| + p(\varepsilon) v(\varepsilon) \\
    & = -|f(x) - f(\bar{x})| + 2 \frac{\sup_{x \in S(\varepsilon)}\{|f(x) - f(\bar{x})|\}}{v(\varepsilon)} v(\varepsilon) \\
    & = \sup_{x \in S(\varepsilon)} \{| f(x) - f(\bar{x}) |\} > 0
\end{split}
\end{equation}
If $x \in T(v(\varepsilon), \varepsilon)$ then:
\begin{equation}
\begin{split}
    P(x, p) - P(\bar{x}, p) & = f(x) + pg(x) - f(\bar{x}) - pg(\bar{x}) \\
    & = f(x) - f(\bar{x}) + pg(x) \\ 
    & \geq v(\varepsilon) + pg(x) > 0 \\
\end{split}
\end{equation}
Finally, for all $x \in P(v(\varepsilon), \varepsilon) \cup T(v(\varepsilon), \varepsilon) = S(\varepsilon)$ then $P(x, p) > P(\bar{x}, p)$, for all $p \geq p(\varepsilon)$.    

We will now analyse the inverse, namely the smallest epsilon, such that a given $p$ gives us $P(x, p) > P(\bar{x}, p)$, for all $x \in S(\epsilon)$.
Let us define the function $e$ as follows:
\begin{equation}
    e(p) = \inf\{\xi \;|\; p(\xi) \leq p\}
\end{equation}
for $p > p(1)$ and $p$ is defined as before. We shall prove that:
\begin{equation}
    e(p) > 0 \quad\text{for}\quad p > p(1) \quad\text{and}\quad \lim_{p \uparrow \infty} e(p) = 0
\end{equation}
Suppose $e(p_0) = 0$ for some $p_0 > 0$. Then there exist $\{\xi_k\}_{k=0}^\infty$ such that:
\begin{equation}
    \lim_{k \rightarrow \infty} \xi_k = 0 \quad\text{and}\quad p(\xi_k) \leq p_0 \quad\text{for all}\quad k \in \mathbb{N}
\end{equation}
from definition of $p(\varepsilon)$:
\begin{equation}
    \lim_{k \rightarrow \infty} \xi_k = 0 \quad\text{and}\quad 2\frac{\sup_{x\in S(\xi_k)}\{|f(x) - f(\bar{x})|\}}{v(\xi_k)} \leq p_0 \quad\text{for all}\quad i \in \mathbb{N}
\end{equation}
\begin{equation}
    \lim_{k \rightarrow \infty} \xi_k = 0 \quad\text{and}\quad 2\frac{\sup_{x\in S(\xi_k)}\{|f(x) - f(\bar{x})|\}}{p_0} \leq v(\xi_k) \quad\text{for all}\quad i \in \mathbb{N}
\end{equation}

Now we construct a sequence $\{x_k\}_{k=0}^\infty$ such that $x_k \in S(\xi_k)$ and:
\begin{equation}
    g(x_k) \geq v(\xi_k) \quad\text{or}\quad f(x_k) - f(\bar{x}) \geq v(\xi_k)
\end{equation}
So now, I do not think that Pietrzykowski is right about the first thing, since $v(\xi_k)$ is not bounded from below, as he suggests. 

Does $e$ converge to $0$? By construction, if $p_1 < p_2$ then:
\begin{equation}
    \{\xi \;|\; p(\xi) \leq p_1\} \subseteq \{ \xi  \;|\; p(\xi) \leq p_2 \}
\end{equation}
and therefore:
\begin{equation}
    \inf\{\xi \;|\; p(\xi) \leq p_1\} \geq \inf\{ \xi  \;|\; p(\xi) \leq p_2 \}
\end{equation}
so $e$ is non-increasing. It is also true that for all $\varepsilon$:
\begin{equation}
    e(p(\varepsilon)) = \inf\{\xi \;|\; p(\xi) \leq p(\alpha) \} \leq \varepsilon
\end{equation}
then $e(p(\varepsilon))$ converges to $0$ with $\varepsilon$.

If $e(p) = 0$ then equivalently $\inf\{\xi \;|\; p(\xi) \leq p\} = 0$ and:
\begin{equation}
\end{equation}

\end{proof}
